# Supplementary material for: DeepLSH: Deep Locality-Sensitive Hash Learning for Fast and Efficient Near-Duplicate Crash Report Detection
Source: arXiv:2310.06703 source file (2023-10-10)
Supplement: Supplementary file 1 [file appendix.tex]

\subsection{Supplementary Materials}\label{appendix:suppMat}
\smallbreak
\noindent \textbf{Comparison between Locality-sensitive hashing and Learn to hash and DeepLSH.} We provide in Table~\ref{tab:comparisonLSH&DH} a detailed comparison between the two hashing techniques: Locality sensitive hashing and Learn to hash and also highlight how \texttt{DeepLSH} can take advantage of the strengths of each technique and overcome their shortcomings. LSH is a hash table lookup strategy that shows superiority in terms of computational time and space complexity since we typically store pointers to data in hash tables. The major advantage of LSH is the ability to provide theoretical guarantees on the search accuracy while having the key hyperparameters $L$ and $K$ to control recall/accuracy trade-off. Nevertheless, considering that LSH is a concept that is fundamentally based on a probabilistic model, it remains difficult and challenging to find for each similarity metric or a newly designed distance, a family of hash functions that satisfies the locality-sensitive property. Moreover, LSH is a data-independent approach i.e.,  it does not adapt to the data-dependent distribution of similarity values. On the other hand, Learn to hash has recently emerged to address these drawbacks of LSH by proposing an end-to-end hashing strategy to learn complex and non-linear similarity functions. However, unlike LSH, we have no guarantees on the search performances, and there is no systematic and universal procedure to generate hash tables such that the probability of two data items being found in the same hash bucket is given as a monotonic function of their similarity value. Hence, \texttt{DeepLSH} has been proposed in this paper to overcome these drawbacks. We perform a hash vector learning process, but in such a way that it converges to the guarantees provided by LSH. \texttt{DeepLSH} learns very complex similarity measures by adapting to the data distribution, but still aims to preserve the locality-sensitive property and not only to mimic the similarity.        

\smallbreak
\noindent \textbf{Proof of property~\eqref{eq:relationProbSim}}. We prove that the probability of two stack traces $s$ and $s'$ to be hashed in the same hash bucket for at least on of the hash tables given the LSH hyperparameters $(L,K)$ is given as: $P_{K,L} (s,s')=1-(1-sim(s,s')^K)^L$.
\begin{align}
&P_{K,L} (s,s')= Pr(s \text{ and } s' \text{ are identical in $1$ hash table}) \nonumber \\
&= 1 - Pr(s \text{ and } s' \text{ are not identical in all $L$ hash tables}) \nonumber \\
&= 1 - Pr(s \text{ and } s' \text{ are not identical in one hash tables})^L \nonumber \\
&= 1 - Pr(s \text{ and } s' \text{ have  $1$ dissimilar meta-hash code})^L \nonumber \\
&= 1 - [1 - Pr(s \text{ and } s' \text{ have the same meta-hash code})]^L \nonumber \\
&= 1 - [1 - Pr(s \text{ and } s' \text{ have the same hash function})^K]^L \nonumber \\
&= 1 - [1 - Pr[h(s) = h(s')]^K]^L \nonumber 
\end{align}
Referring to Property~\eqref{eq:collisionProb}, and assuming that: $g(x) = I_x$ i.e. $Pr[h(s) = h(s')] = sim(s,s')$, we have: 
\begin{align}
P_{K,L} (s,s')&= 1 - [1-sim(s,s')]^K]^L \nonumber 
\end{align}

\smallbreak
\noindent \textbf{Feature encoding architecture.} As explained in Subsection~\ref{subsec:learnLSH}, we leverage a CNN-based stack trace encoder. This choice can be justified by the capability of the CNN model to efficiently encode data items while preserving the order, importance, and relevance of each frame w.r.t. the output (i.e., the computed similarity value) by contextualizing it within an ordered set of frames. This set is specified through the size of the filters, taking $3$ different sizes of kernels, which is similar to reproducing N-grams with different values of N. $1-$Max pooling is applied on each convolution stack to extract the largest number for each filter as a representative feature map that are concatenated in a single univariate vector that is fed to the multi-layer perceptron hash model.       

\smallbreak
\noindent \textbf{Examples on the generalized Hamming similarity.} In the following, we show through two similar examples in Figure~\ref{fig:exampleHam} with different parameters of the number of hash functions $M$ and size of hash function $b$, how the generalized Hamming similarity is calculated as indicated in the formula~\eqref{eq:Hammingcase1}. Consider example 1, where the size of a hash function is defined on 2 bits, thus two hash functions are considered similar if all $b$ bits are identical, i.e. $D_{\text{Chebyshev}}(h_k^i ,h_k^j) = 0$. The generalized Hamming similarity is then calculated as follows: 
$gHam \left(H(s_i), H(s_j)\right) = 1 - \frac{max(2,2) + max(0,0) + max(2,0)}{2 \cdot 3} = 1 - \frac{4}{6} = \frac{1}{3}$. The same hash vectors have a different value of the generalized Hamming similarity when $b = 1$, corresponding to the well-known Hamming similarity calculated for $1$ bit.   
\begin{figure}[h]
\centering
 \includegraphics[width=0.45\textwidth]{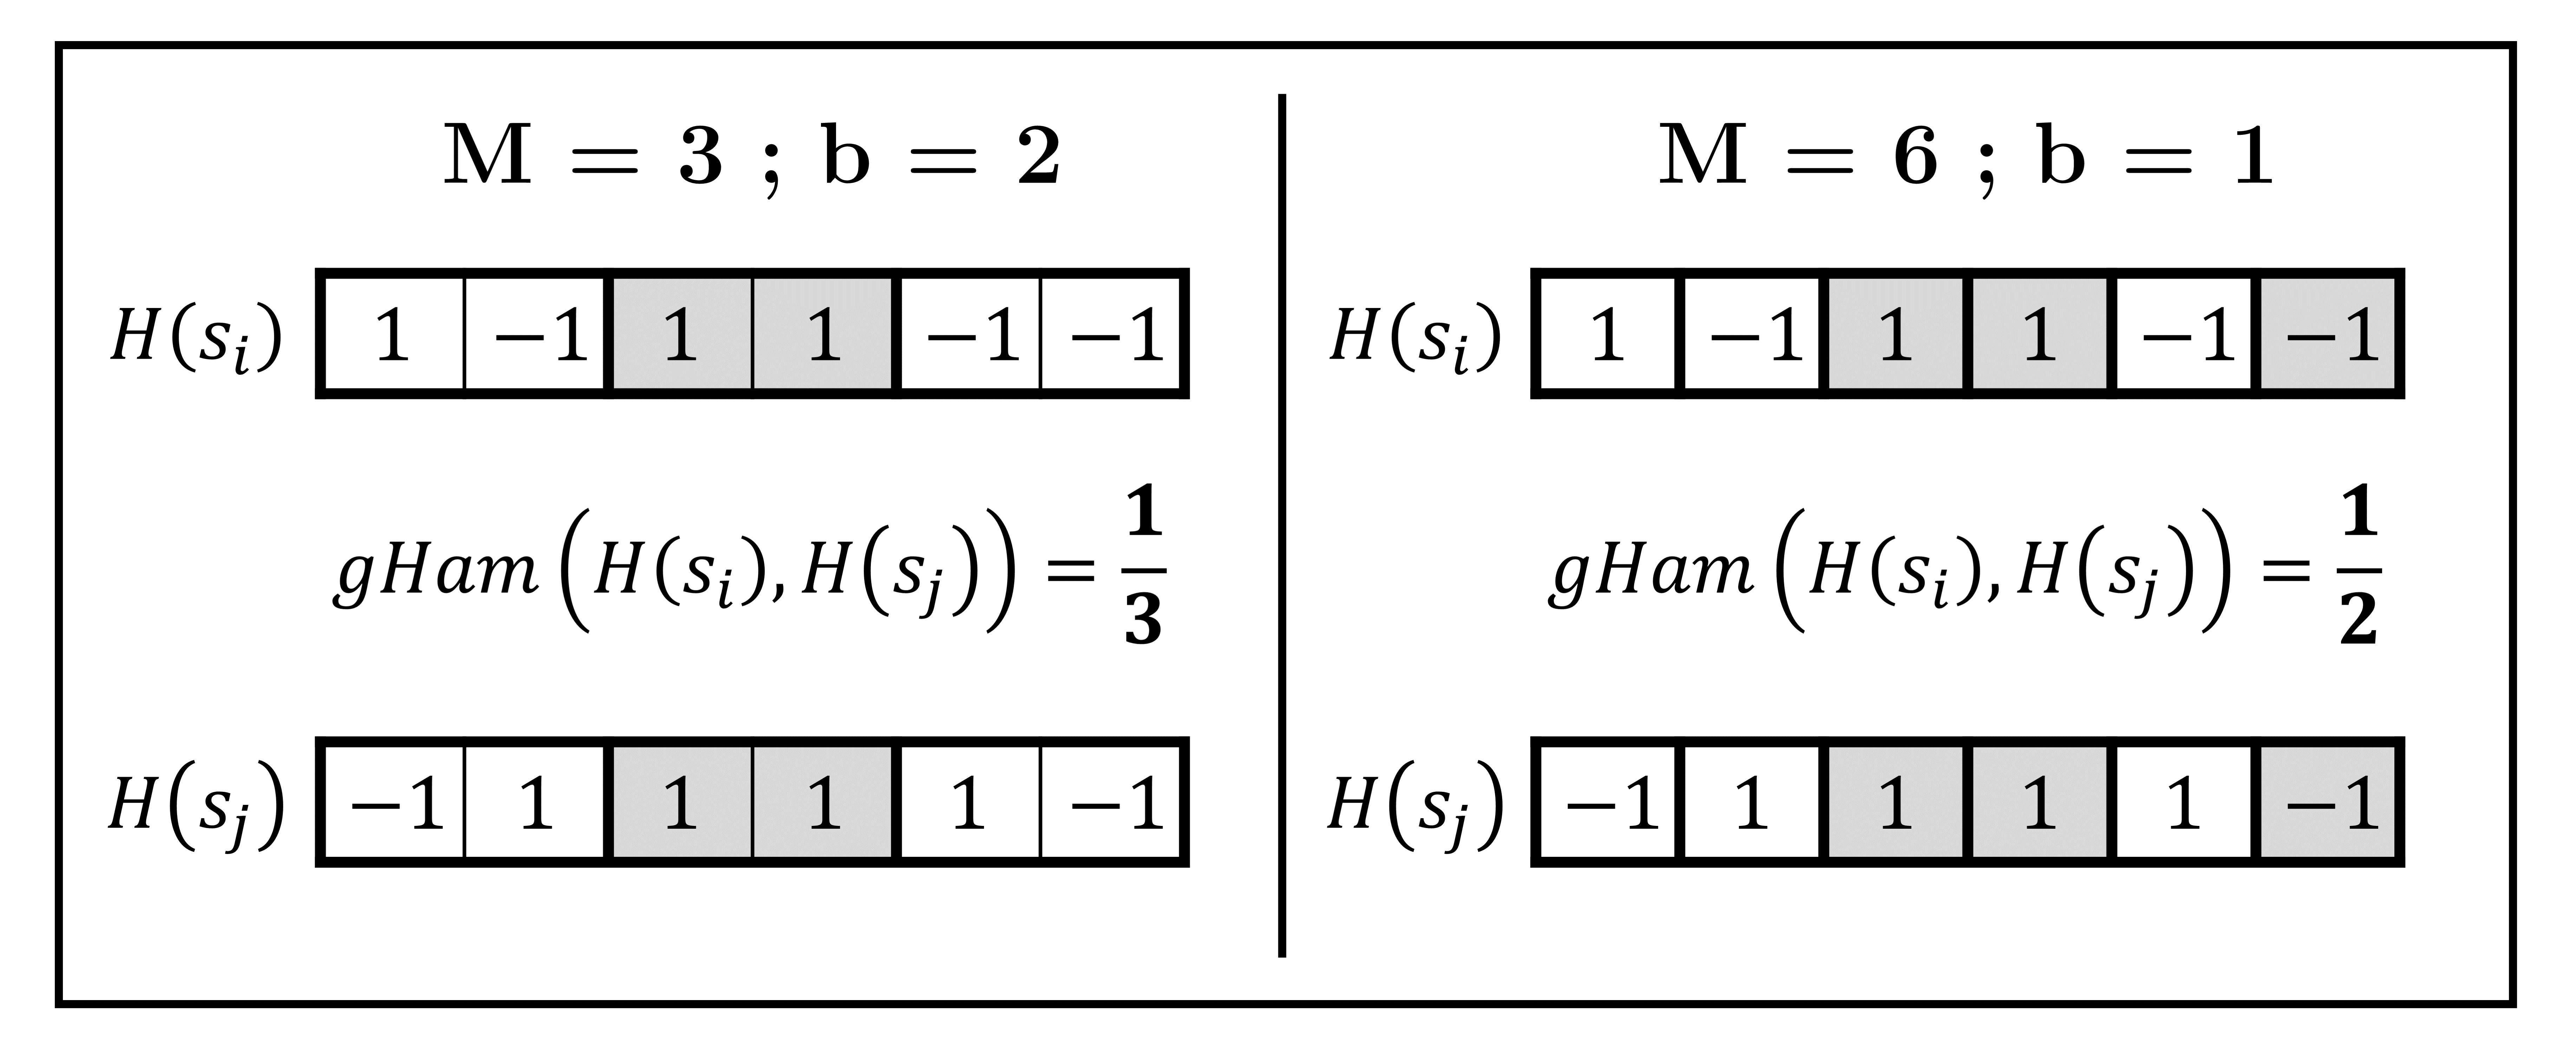}
\caption{\label{fig:exampleHam} \small (Appendix) Examples of the generalized Hamming similarity with different values of $M$ and $b$.}
\end{figure}

\subsection{Supplementary Experiments}

\smallbreak

\noindent \textbf{Distributions of similarity values  w.r.t. similarity measures.} As shown previously in Figure~\ref{fig:distSim}, the correlation between the similarity measures is relatively low. We also study the distribution of similarity values greater than 0.5 (i.e., we take only the large similarity values that are likely to be near-duplicate candidates). We observe that the distributions are quite different, and have various shapes, which again demonstrates that \texttt{DeepLSH} model has been trained on different samples of pairwise similarities.

\begin{figure}[t]
\centering
 \includegraphics[width=0.5\textwidth]{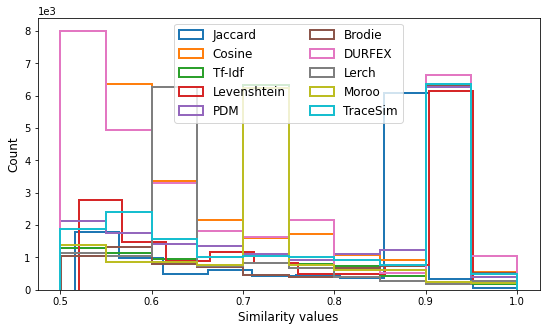}
\caption{\label{fig:distSim} \small (Appendix) Comparison between the distributions of similarity values (greater than $0.5$) for all used similarity measures.} 
\end{figure}
