# Supplementary material for: DeepLSH: Deep Locality-Sensitive Hash Learning for Fast and Efficient Near-Duplicate Crash Report Detection
Source: arXiv:2310.06703 source file (2023-10-10)
Supplement: Supplementary file 2 [file materialsAppendix.tex]

\begin{table*}[t]
    \centering
    \caption{\small (Appendix) Comparison between Locality-sensitive hashing and Learn to hash.}
    
    \scalebox{0.9}{
    \begin{tabular}{c|l|l}
    \toprule
              \textbf{Technique} & \multicolumn{1}{c|}{\textbf{Locality Sensitive Hashing (LSH)}}                                                                                                                                                                & \multicolumn{1}{c}{\textbf{Learn to Hash}}                                                                                                                                                    \\ \midrule
    \textbf{\textcolor{PineGreen}{Strengths}}  & \begin{tabular}[c]{@{}l@{}}\textcolor{PineGreen}{+} \textbf{Superiority} in computational \textbf{time complexity} and \textbf{storage}\\ \textcolor{PineGreen}{+} Theoretical \textbf{guarantees} on search accuracy\\ \textcolor{PineGreen}{+} Provide an \textbf{efficient search schemes} rooted in \textbf{hash tables}\end{tabular} & \begin{tabular}[c]{@{}l@{}}\textcolor{PineGreen}{+} \textbf{End-to-end} hashing codes\\ \textcolor{PineGreen}{+} Learn \textbf{complex and non-linear similarity functions}\\ \textcolor{PineGreen}{+} Data \textbf{dependant}\end{tabular}                                                                 \\ \midrule
    \textbf{\textcolor{red}{Weaknesses}} & \begin{tabular}[c]{@{}l@{}}\textcolor{red}{-} Difficult to derive \textbf{LSH families} for any \textbf{custom} similarity measure\\ \textcolor{red}{-} Data \textbf{independent} (does not fit with \textbf{data distributions})\end{tabular}                                       & \begin{tabular}[c]{@{}l@{}}\textcolor{red}{-} Challenging problem of learning \textbf{binary} codes\\ \textcolor{red}{-} \textbf{No guarantees} on the search accuracy\\ \textcolor{red}{-} \textbf{No systematic procedure} to construct hash tables\end{tabular} \\ \bottomrule
    \end{tabular}}
    \label{tab:comparisonLSH&DH}
\end{table*}

\begin{figure*}
\centering
 \includegraphics[width=0.92\textwidth]{}% &
\caption{\label{fig:modelF} \small (Appendix) A detailed schematic illustration of the employed model architecture.}
\end{figure*}
